# Supplementary material for: Mirrored Langevin Dynamics
Source: arXiv:1802.10174 source file (2020-12-30)
Supplement: Supplementary file 1 [file appendixA.tex]

\section{Properties of $\Lh$}

Let $\ip{\cdot}{\cdot}_M$ be a Riemannian metric \citep{lee2006riemannian}. We use $\Delta_M$ and $\nabla_M$ to denote the Laplace-Beltrami operator and Riemannian gradient, respectively.

The following results (some without proof) were announced in \citep{kolesnikov2014hessian}. We provide the proof for completeness.

\begin{lemma}[Properties of $\L_h$]\label{lem:properties_Lh}
\begin{enumerate}
\item $\L_h$ admits the following equivalent formulation:
\begin{align}
\Lh f &= \Tr \nabla^2 h^{-1} \nabla^2 f - \ip{\nabla W \circ \nabla h}{\nabla f} \label{eq:diffusion_equivalent1}\\
&= \Div_\nu\l( \nabla f \circ \nabla \hstar  \r) \circ \nabla h.\label{eq:diffusion_equivalent2}
\end{align}
%Here, $\Delta_M$ denotes the Laplace-Beltrami operator, $\nabla_M$ denotes the 
\item $\L_h$ is symmetric in $\mathbb{L}_2$ with respect to $\mu$:
\beq \label{eq:Lh_symmetric}
\forall f, g \in \Cc \quad \int f \L_h g d\mu = \int g \L_h f d\mu.
\eeq

\item The following differential equation holds for all directions $\mathbf{e} \in \RR^d$:
\beq \label{eq:Lh_differential_equation}
\partial_{\mathbf{e}} V = - \L_h (\partial_{\mathbf{e}} h).
\eeq
In particular, we have 
\beq  \nn
\nabla V = - \L_h (\nabla h)
\eeq
where $\L_h$ applies coordinate-wise to $\nabla h$.

\item The dual diffusion operator $\mathcal{L}_{\hstar}$, defined by $\mathcal{L}_{\hstar} f\coloneqq  \Div_\mu\l(  \nabla f\circ \nabla h \r) \circ \nabla \hstar$ for all $f\in \Cc$, satisfies the dual differential equation of \eqref{eq:Lh_differential_equation}
\beq \label{eq:Lh_differential_equation_dual}
\partial_{\mathbf{e}} W = - \mathcal{L}_{\hstar} (\partial_{\mathbf{e}} \hstar).
\eeq

\item Consider the weighted Riemannian manifold $(\RR^d, \nabla^2 h, \mu)$. Then an alternative expression for $\Lh$ is
\beq 
\Lh = \Delta_M f - \ip{\nabla_M P}{\nabla_M f}_M, 
\eeq
where $P = \frac{1}{2}\l( V + W\circ \nh\r).$
\end{enumerate}
\end{lemma}

\begin{proof}
\begin{enumerate}
\item We depart from the expression \eqref{eq:diffusion_equivalent1}: $\Lh f= \Div_\nu\l( \nabla f\circ \nhstar \r) \circ \nh.$ Composing both sides with $\nhstar$, we get
\begin{align}
(\Lh f) \circ \nhstar (\x)&= \Div_\nu\l( \nabla f\circ \nhstar \r)(\x) \nn\\
&= \Div\l( \nabla f\circ \nhstar \r)(\x)  - \ip{\nabla W(\x)}{ (\nabla f \circ \nhstar)(\x)}\nn \\
&= \sum_{i=1}^d \frac{\partial}{\partial x_i} \l( \nabla f\circ \nhstar \r)_i (\x)  - \ip{\nabla W (\x)}{( \nabla f \circ \nhstar)(\x)}. \label{eq:proof_Lh_hold1}
\end{align}Noticing that $\l( \nabla f\circ \nhstar \r)_i = \partial_i f \circ \nhstar$, we get, with $\mathbf{e}_i$'s denoting the standard basis for $\RR^d$,
\begin{align}
\sum_{i=1}^d \frac{\partial}{\partial x_i} \l( \nabla f\circ \nhstar \r)_i (\x) \nn&=
 \sum_{i=1}^d \frac{\partial}{\partial x_i} \l( \partial_i f \circ \nhstar \r) (\x) \nn\\
&= \sum_{i=1}^d  \ip{\nabla^2 \hstar(\x) \cdot (\nabla \partial_i f \circ \nhstar) (\x)}{\mathbf{e}_i} \nn\\
&= \sum_{i=1}^d  \ip{  (\nabla \partial_i f \circ \nhstar) (\x)}{\nabla^2 \hstar(\x)\mathbf{e}_i} \nn \\
&= \sum_{i=1}^d  \ip{  \mathbf{e}_i^\top (\nabla^2  f \circ \nhstar) (\x)}{\nabla^2 \hstar(\x)\mathbf{e}_i} \nn\\
&= \Tr \nabla^2 \hstar(\x) \cdot(\nabla^2  f \circ \nhstar) (\x). \label{eq:proof_Lh_hold2}
\end{align}Substituting \eqref{eq:proof_Lh_hold2} into \eqref{eq:proof_Lh_hold1}, composing both sides by $\nh$, and using $\nabla^2 \hstar \circ \nh = \nabla^2 h^{-1}$, we get
\begin{align*}
\Lh f= \Tr \nabla^2 h^{-1} \nabla^2 f - \ip{\nabla W \circ \nh}{ \nabla f }
\end{align*}which proves \eqref{eq:diffusion_equivalent2}=\eqref{eq:diffusion_equivalent1}.

\item Recall that $\nh \# \mu = \nu$ if and only if $\nhstar \# \nu = \mu$. We write, for all $f$ and $g\in\Cc$,
\begin{align}
\int f\Lh g \dmu &= \int f \cdot \Div_\nu\l(  \nabla g \circ \nhstar \r) \circ \nh \dmu \nn\\
&= \int ( f\circ \nhstar) \cdot\Div_\nu \l(  \nabla g \circ \nhstar \r)  \dnu  && \textup{by \eqref{eq:push_forward} for $\nh \# \mu = \nu$} \nn \\
&= -\int \ip{\nabla ( f\circ \nhstar) }{ \nabla g \circ \nhstar} \dnu && \textup{by \eqref{eq:weighted_divergence}} \nn \\
&=  -\int \ip{\nabla^2 \hstar \cdot( \nabla f\circ \nhstar) }{ \nabla g \circ \nhstar} \dnu \nn \\
&= -\int \ip{\nabla f\circ \nhstar }{ \nabla^2 \hstar \cdot (\nabla g \circ \nhstar)}  \dnu \nn \\
&= -\int \ip{\nabla f\circ \nhstar }{  \nabla( g \circ \nhstar)}  \dnu \nn \\ 
&= \int \Div_\nu ( \nabla f\circ \nhstar) \cdot  \l(g \circ \nhstar  \r)\dnu &&  \textup{by \eqref{eq:weighted_divergence}} \nn \\
&= \int g \cdot \Div_\nu\l(  \nabla f \circ \nhstar \r) \circ \nh \dmu \nn  && \textup{by \eqref{eq:push_forward} for $\nhstar \# \nu = \mu$} \nn  \\
&= \int g\Lh f \dmu. \nn
\end{align}

\item By the Monge-Amp\'ere equation \eqref{eq:Monge-Ampere}, we have
\beq \label{eq:proof_Lh_hold3}
V = W \circ \nh - \log \det \nabla^2 h.
\eeq

Given any $\mathbf{e} \in \RR^d$, we differentiate both sides of \eqref{eq:proof_Lh_hold3} in the direction of $\mathbf{e}$ to yield
\begin{align*}
\partial_{\mathbf{e}} V &= \ip{\nabla^2 h \cdot \l(  \nabla W \circ \nh \r)}{\mathbf{e}} - \Tr \nabla^2 h^{-1} \nabla^2 \l(\partial_{\mathbf{e}} h \r) \\
&=\ip{  \nabla W \circ \nh }{\nabla^2 h \cdot \mathbf{e}} - \Tr \nabla^2 h^{-1} \nabla^2 \l(\partial_{\mathbf{e}} h \r) \\
&= \ip{  \nabla W \circ \nh }{\nabla  \l(\partial_{\mathbf{e}} h\r)} - \Tr \nabla^2 h^{-1} \nabla^2 \l(\partial_{\mathbf{e}} h \r) \\
&= - \Lh \l(\partial_{\mathbf{e}} h\r).
\end{align*}

\item Recall that $\nh \# \mu = \nu$ if and only if $\nhstar \# \nu = \mu$. Now switch the role of $W$ and $V$.

\item The proof involves the theory of Riemannian Dirichlet forms; we refer to \citep{bakry2013analysis} and \citep{kolesnikov2014hessian} for details. 
\end{enumerate}
\end{proof}
